# Supplementary material for: Tracing the Propagation Path: A Flow Perspective of Representation Learning on Graphs
Source: arXiv:1912.05977 source file (2019-12-12)
Supplement: Supplementary file 1 [file graph19-0appendix.pdf]

# 7 Appendix

## 7.1 Proof of Theorem 4.1

To prove Theorem 4.1, we describe some preliminaries. Our proof partially relies on the results given by [24], where the authors . For completeness, we give the definition of influence distribution and the theorem.

**Definition 7.1** (Influence score and distribution)**.** Given a graph $\mathcal{G}(\mathcal{V}, \mathcal{E})$, let $h_x^{(0)}$ be the input feature and $h_x^{(k)}$ be the learned hidden feature of node $x \in \mathcal{V}$ at the k-th layer of the model. The *influence score* $I(x, y)$ of node $x$ by any node $y \in \mathcal{V}$ is the sum of the absolute values of the entries of the Jacobian matrix $[\frac{\partial h_x^{(k)}}{\partial h_y^{(0)}}]$. We define the *influence distribution* $I_x$ of $x \in \mathcal{V}$ by normalizing the *influence scores*: $I_x(y) = I(x, y)/\sum_z I(x, z)$, or $I_x(y) = e^T[\frac{\partial h_x^{(k)}}{\partial h_y^{(0)}}]e/(\sum_{z \in V} e^T[\frac{\partial h_x^{(k)}}{\partial h_z^{(0)}}]e)$, where $e$ is the all-ones vector.

**Theorem 7.1.** *Given a k-layer GCN with averaging as its neighborhood aggregation scheme, assume that all paths in the computation graph of the model are activated with the same probability of success $\rho$. Then the influence distribution $I_x$ for any node $x \in \mathcal{V}$ is equivalent, in expectation, to the $k$-step random walk distribution on the same graph stating at node $x$.*

Below we restate the Theorem 4.1 and provide a proof.

**Theorem 4.1.** *Given a grid graph $\mathcal{G}(\mathcal{V}, \mathcal{E})$, and a k-layer GCN with averaging as its neighborhood aggregation scheme, there exists an equivalent version of FlowGN that has the same influence distribution for every node $x \in \mathcal{V}$.*

*Proof.* We prove Theorem 4.1 in three steps. First, we prove that the influence distribution of a k-layer GCNs with averaging as its neighborhood aggregation scheme is equivalent to a k-step random walker with uniform transition probabilities. This can directly inferred from Theorem 7.1 and its proof [24].

Second, a random walker with uniform transition probabilities in a grid graph indicates that every node has a same number of neighbors and a same transition probability to its neighbors. In other words, the random walker is symmetric and so is the related influence distribution of GCNs, i.e, $I_x(y) = I_y(x)$.

Third, we prove that there exists a one-layer FlowGN that its influence distribution is equivalent to a k-step random walker. We can set the return parameter $p = 1$, the in-out parameter $q = 1$, and the path length $l = k$ so the generated flow paths are exactly a sampling of a k-step random walker (in grid graphs the importance of all nodes are the same in a structural view). We apply the same information propagation mechanism used in the experiments, i.e., $GenerateFlow(s) = h_s$, $TransmitFlow(v_i, flow) = flow$, and $ConserveFlow(v_i, flow) = flow$. For clarification, we set *source* node as $y$ and *sink* node as $y$. Following the proof procedure of Theorem 7.1 [24], we can draw that $E[\frac{\partial h_y^{(k)}}{\partial h_x^{(0)}}] = \rho \cdot W \cdot (\prod_{p=1}^{\Phi} \prod_{l=k}^{1} \frac{1}{\widetilde{deg}(v_p^l)})$. By normalizing the distribution scores, we can get that the influence distribution $I_x(y)$ of FlowGN is equivalent to a random walker that starts at node $y$. Since $I_x(y) = I_y(x)$, we get the Theorem proved.

□

## 7.2 Experimental Details

We used TensorFlow for all experiments except SGC, which is implemented by Pytorch. Running time is compared on a single machine with 4-core 2.2 GHz Intel Core i7, and 16G RAM. For FlowGN, we set weight decay to 0.00001, epochs to 30 hidden and out dimensions to 50 The early stopping criterion uses a patience of $p = 10$ and epochs is set to 100. The learning rate is set to 0.0001.

We mainly use the original parameters for baselines. The vanilla GCN uses the original settings of two layers with $h = 16$ hidden units, no dropout on the adjacency matrix, $L_2$ regularization parameter $\lambda = 5 \times 10^{-4}$ and the original early stopping with a maximum of 200 steps and a patience of 10 steps based on the loss. The batch version of GCN is the same as the one used by FastGCN. For GAT

and SGC, we use the (well optimized) original hyperparameters. For GraphSAGE, we set batch size to $256$ and dropout to $0$. In Section 5.3, due to memory limit, we set the sampling size to $5$ and batch size to $50$ for all layers when model depth exceeds $5$. For FastGCN, the sampling size is set to $400$.

### 7.3 Additional Experimental Results

Results of Cora are shown in Figure 4 and Figure 5. The optimal $l$ is $6$ and optimal $q$ is $0.1$, and we can get similar conclusion as what we made in Section 5.2.

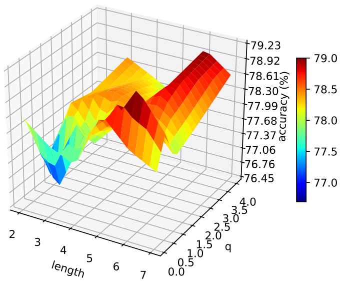


(a) Cora

Figure 4: Prediction accuracy of FlowGN with different path length $l$ and in-out parameter $q$.

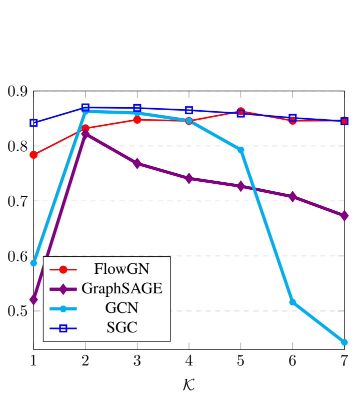


Figure 5: Prediction accuracy of FlowGN on *Cora* with different layer numbers $\mathcal{K}$
